# Supplementary material for: First Measurement of Inclusive Muon Neutrino Charged Current Differential Cross Sections on Argon at $E_\nu \sim 0.8$ GeV with the MicroBooNE Detector
Source: arXiv:1905.09694 ancillary file (2019-09-30)
Supplement: Supplementary file 1 [file supplemental_material.pdf]

# Supplementary Material: First Measurement of Inclusive Muon Neutrino Charged Current Differential Cross Sections on Argon at $E_\nu \sim 0.8$ GeV

(Dated: July 30, 2019)

## SMEARING MATRIX

The smearing matrix $S$ transforms the number of generated events $N_j^{\text{gen}}$ in a bin $j$ of generated momentum and angle to the number of events $N_i$ in a bin $i$ of measured momentum and angle. In the analysis, the smearing matrix is used to transform the selection efficiency from a function of generated momentum and angle to a function of measured momentum and angle. $S$ is also needed to transform any cross section model prediction reported as a function of true kinematic variables into a function of measured kinematic variables that can be compared to the MicroBooNE data. The bin content in a bin $i$ of measured kinematics is given as $N_i = \sum_{j=1}^{M} S_{ij} N_j^{\text{gen}}$ where the entries of $S$ are defined as $S_{ij} = P(\text{measured in bin}\, i \,|\, \text{generated in bin}\, j)$ and $M$ is the total number of bins. The binning chosen in this analysis is illustrated in Fig. 1. The smearing matrix is shown in Fig. 2 with entries for all 42 bins used in the double differential cross section calculation and an additional bin representing the overflow. The red lines mark boundaries between different slices in $\cos\theta_\mu$. Within each slice, the muon momentum $p_\mu$ is increasing with increasing bin number. The values of the smearing matrix are provided in the attached text file `microboone_cc_inclusive_smearing_matrix.txt`.

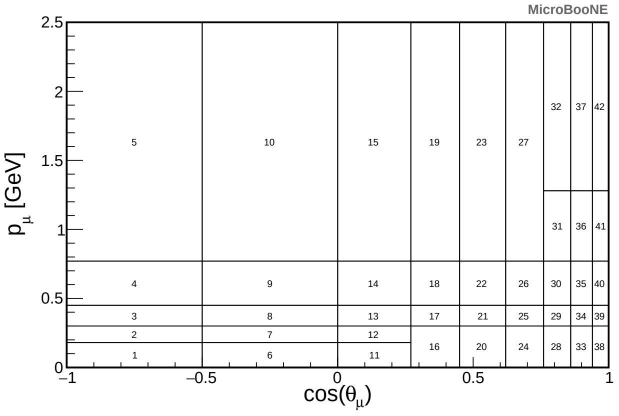


FIG. 1. Bin definitions for the double-differential cross section measurement in the phase space of measured muon momentum and angle.

## COVARIANCE MATRIX

The total covariance matrix $E$ obtained in the measurement is shown in Fig. 3. $E$ consists of the statistical and systematic uncertainties, $E = E^{\text{stat}} + E^{\text{syst}}$. The binning is defined as illustrated in Fig. 1. The values of the covariance matrix are provided in the attached text file `microboone_cc_inclusive_covariance_matrix.txt`.

## CROSS SECTION VALUES

Table I shows the double-differential cross section result for the 42 bins in muon momentum and muon angle used in this measurement. The table also specifies the bin number and ranges for each of the 42 bins in the first three columns. The $\nu_\mu$ charged current inclusive cross section is given per nucleon. We also give the total uncertainty in each bin, which is obtained from the diagonal elements of the covariance matrix (see Fig. 3). The last columns shows the selection efficiency folded with the acceptance that applies to each bin. The values of the cross section are provided in the attached text file `microboone_cc_inclusive_cross_section.txt`.

## BNB FLUX PREDICTION

The flux prediction for $\nu_\mu$ from the Booster Neutrino Beam (BNB) at MicroBooNE is listed in Table II as a function of the neutrino energy $E_\nu$. The values of the flux are provided in the attached text file `microboone_cc_inclusive_flux.txt`.

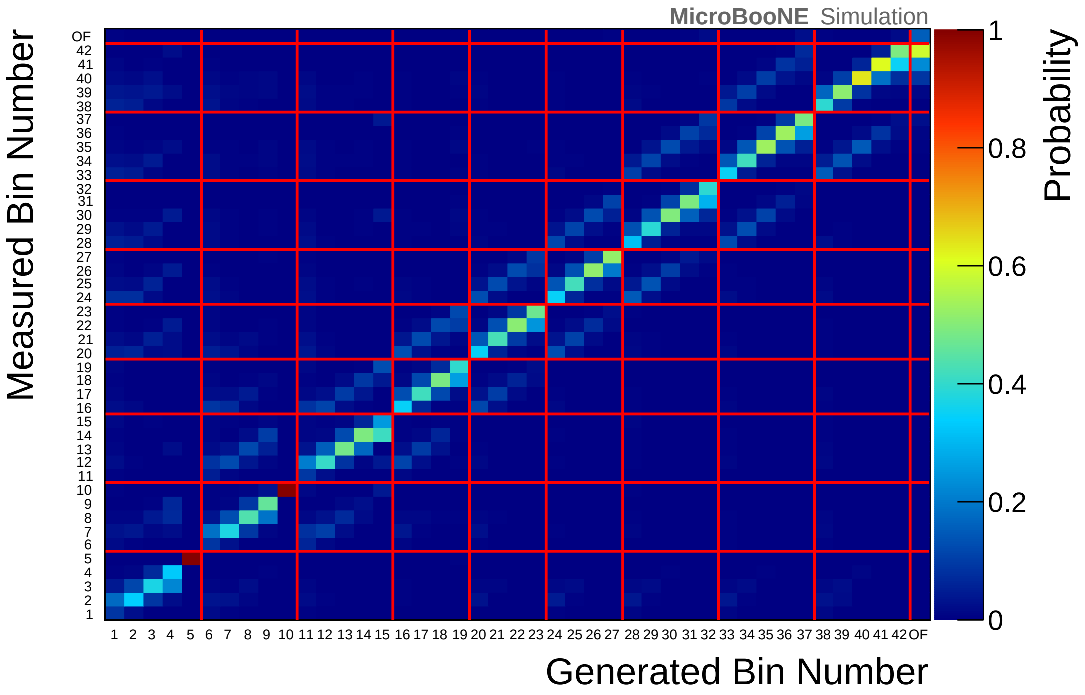


FIG. 2. Migration matrix for the $p_\mu$ and $\cos\theta_\mu$ distributions. The color scale represents the probability that an event in generated bin $j$ is observed in the bin of measured kinematics $i$. The bin denoted with "OF" is the overflow bin in the muon momentum distribution.

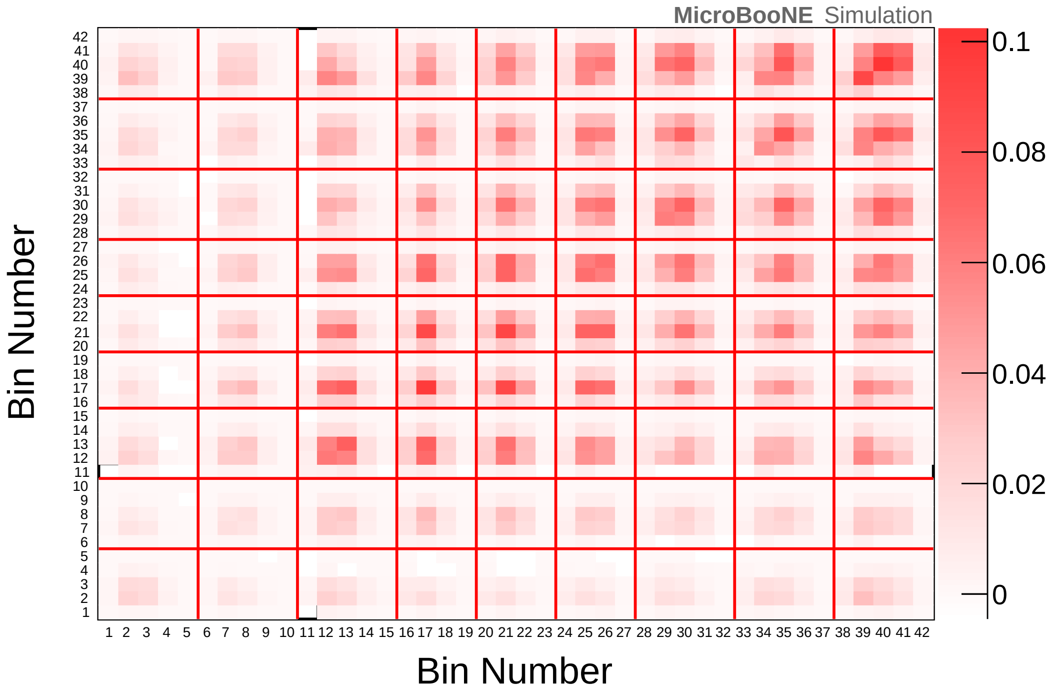


FIG. 3. The total covariance matrices showing both statistical and systematic uncertainties for the double-differential cross section results with 42 bins in the parameter space of measured muon momentum $p_\mu$ and cosine of the muon angle $\cos\theta_\mu$.

TABLE I. $\nu_\mu$ charged current inclusive cross section per nucleon in each measurement bin with total statistical plus systematic uncertainty. Negative values of the cross section are possible and reflect that mean expected background is larger than the data measurement for those particular bins. For these bins the measured values are consistent with zero. The total uncertainty comes from the square-root of the covariance matrix diagonal entries. Columns 2 and 3 show the ranges for each of the 42 bins in the measurement. Column 6 lists the selection efficiency times acceptance per bin.

| Bin Number | $\cos\theta_\mu$ Range | $p_\mu$ Range [GeV] | $d^2\sigma/dp_\mu d\cos\theta_\mu$ [$10^{-38}$cm$^2$/GeV] | Total Uncertainty [$10^{-38}$cm$^2$/GeV] | Efficiency |
|---|---|---|---|---|---|
| 1 | [-1.00, -0.50) | [0.00, 0.18) | $3.8 \times 10^{-2}$ | $3.8 \times 10^{-2}$ | 0.30 |
| 2 | [-1.00, -0.50) | [0.18, 0.30) | $2.5 \times 10^{-1}$ | $1.5 \times 10^{-1}$ | 0.39 |
| 3 | [-1.00, -0.50) | [0.30, 0.45) | $2.2 \times 10^{-1}$ | $1.3 \times 10^{-1}$ | 0.47 |
| 4 | [-1.00, -0.50) | [0.45, 0.77) | $4.1 \times 10^{-2}$ | $3.6 \times 10^{-2}$ | 0.55 |
| 5 | [-1.00, -0.50) | [0.77, 2.50] | $-0.9 \times 10^{-3}$ | $2.9 \times 10^{-3}$ | 0.52 |
| 6 | [-0.50, 0.00) | [0.00, 0.18) | $1.4 \times 10^{-2}$ | $3.3 \times 10^{-2}$ | 0.32 |
| 7 | [-0.50, 0.00) | [0.18, 0.30) | $2.2 \times 10^{-1}$ | $1.3 \times 10^{-1}$ | 0.41 |
| 8 | [-0.50, 0.00) | [0.30, 0.45) | $2.9 \times 10^{-1}$ | $1.3 \times 10^{-1}$ | 0.47 |
| 9 | [-0.50, 0.00) | [0.45, 0.77) | $5.9 \times 10^{-2}$ | $3.4 \times 10^{-2}$ | 0.46 |
| 10 | [-0.50, 0.00) | [0.77, 2.50] | $-0.2 \times 10^{-3}$ | $3.2 \times 10^{-3}$ | 0.45 |
| 11 | [0.00, 0.27) | [0.00, 0.18) | $-3.1 \times 10^{-2}$ | $7.5 \times 10^{-2}$ | 0.33 |
| 12 | [0.00, 0.27) | [0.18, 0.30) | $4.7 \times 10^{-1}$ | $2.7 \times 10^{-1}$ | 0.44 |
| 13 | [0.00, 0.27) | [0.30, 0.45) | $6.7 \times 10^{-1}$ | $2.8 \times 10^{-1}$ | 0.52 |
| 14 | [0.00, 0.27) | [0.45, 0.77) | $1.3 \times 10^{-1}$ | $0.8 \times 10^{-1}$ | 0.52 |
| 15 | [0.00, 0.27) | [0.77, 2.50] | $-1.1 \times 10^{-2}$ | $2.5 \times 10^{-2}$ | 0.49 |
| 16 | [0.27, 0.45) | [0.00, 0.30) | $2.1 \times 10^{-1}$ | $1.3 \times 10^{-1}$ | 0.44 |
| 17 | [0.27, 0.45) | [0.30, 0.45) | $7.8 \times 10^{-1}$ | $3.2 \times 10^{-1}$ | 0.55 |
| 18 | [0.27, 0.45) | [0.45, 0.77) | $3.5 \times 10^{-1}$ | $1.1 \times 10^{-1}$ | 0.57 |
| 19 | [0.27, 0.45) | [0.77, 2.50] | $-1.3 \times 10^{-2}$ | $2.4 \times 10^{-2}$ | 0.53 |
| 20 | [0.45, 0.62) | [0.00, 0.30) | $2.4 \times 10^{-1}$ | $1.2 \times 10^{-1}$ | 0.46 |
| 21 | [0.45, 0.62) | [0.30, 0.45) | $10.2 \times 10^{-1}$ | $3.1 \times 10^{-1}$ | 0.58 |
| 22 | [0.45, 0.62) | [0.45, 0.77) | $6.4 \times 10^{-1}$ | $1.7 \times 10^{-1}$ | 0.61 |
| 23 | [0.45, 0.62) | [0.77, 2.50] | $1.8 \times 10^{-2}$ | $1.8 \times 10^{-2}$ | 0.57 |
| 24 | [0.62, 0.76) | [0.00, 0.30) | $25.0 \times 10^{-2}$ | $7.9 \times 10^{-2}$ | 0.47 |
| 25 | [0.62, 0.76) | [0.30, 0.45) | $12.5 \times 10^{-1}$ | $2.7 \times 10^{-1}$ | 0.60 |
| 26 | [0.62, 0.76) | [0.45, 0.77) | $11.2 \times 10^{-1}$ | $2.6 \times 10^{-1}$ | 0.63 |
| 27 | [0.62, 0.76) | [0.77, 2.50] | $7.4 \times 10^{-2}$ | $2.2 \times 10^{-2}$ | 0.61 |
| 28 | [0.76, 0.86) | [0.00, 0.30) | $18.1 \times 10^{-2}$ | $7.5 \times 10^{-2}$ | 0.46 |
| 29 | [0.76, 0.86) | [0.30, 0.45) | $9.3 \times 10^{-1}$ | $2.6 \times 10^{-1}$ | 0.60 |
| 30 | [0.76, 0.86) | [0.45, 0.77) | $15.3 \times 10^{-1}$ | $2.8 \times 10^{-1}$ | 0.64 |
| 31 | [0.76, 0.86) | [0.77, 1.28) | $6.9 \times 10^{-1}$ | $1.5 \times 10^{-1}$ | 0.63 |
| 32 | [0.76, 0.86) | [1.28, 2.50] | $3.4 \times 10^{-2}$ | $1.8 \times 10^{-2}$ | 0.60 |
| 33 | [0.86, 0.94) | [0.00, 0.30) | $2.3 \times 10^{-1}$ | $1.1 \times 10^{-1}$ | 0.44 |
| 34 | [0.86, 0.94) | [0.30, 0.45) | $9.6 \times 10^{-1}$ | $2.5 \times 10^{-1}$ | 0.59 |
| 35 | [0.86, 0.94) | [0.45, 0.77) | $18.0 \times 10^{-1}$ | $2.9 \times 10^{-1}$ | 0.65 |
| 36 | [0.86, 0.94) | [0.77, 1.28) | $11.8 \times 10^{-1}$ | $1.8 \times 10^{-1}$ | 0.64 |
| 37 | [0.86, 0.94) | [1.28, 2.50] | $9.7 \times 10^{-2}$ | $1.8 \times 10^{-2}$ | 0.61 |
| 38 | [0.94, 1.00] | [0.00, 0.30) | $1.8 \times 10^{-1}$ | $1.3 \times 10^{-1}$ | 0.43 |
| 39 | [0.94, 1.00] | [0.30, 0.45) | $9.8 \times 10^{-1}$ | $3.2 \times 10^{-1}$ | 0.57 |
| 40 | [0.94, 1.00] | [0.45, 0.77) | $16.9 \times 10^{-1}$ | $3.3 \times 10^{-1}$ | 0.64 |
| 41 | [0.94, 1.00] | [0.77, 1.28) | $13.9 \times 10^{-1}$ | $2.7 \times 10^{-1}$ | 0.62 |
| 42 | [0.94, 1.00] | [1.28, 2.50] | $19.4 \times 10^{-2}$ | $4.5 \times 10^{-2}$ | 0.57 |

TABLE II. The BNB $\nu_\mu$ flux at MicroBooNE corresponding to the differential cross section measurement.

| Energy Range [GeV] | Neutrino Flux [$\nu_\mu$/cm$^2$] | Energy Range [GeV] | Neutrino Flux [cm$^{-2}$] | Energy Range [GeV] | Neutrino Flux [$\nu_\mu$/cm$^2$] | Energy Range [GeV] | Neutrino Flux [$\nu_\mu$/cm$^2$] |
|---|---|---|---|---|---|---|---|
| [0.00, 0.05) | 4.92544e+08 | [1.70, 1.75) | 7.38243e+08 | [3.40, 3.45) | 2.55155e+07 | [5.10, 5.15) | 4.64148e+06 |
| [0.05, 0.10) | 1.89066e+09 | [1.75, 1.80) | 6.11492e+08 | [3.45, 3.50) | 2.48278e+07 | [5.15, 5.20) | 4.45764e+06 |
| [0.10, 0.15) | 2.44421e+09 | [1.80, 1.85) | 5.07337e+08 | [3.50, 3.55) | 2.44332e+07 | [5.20, 5.25) | 4.13457e+06 |
| [0.15, 0.20) | 2.91236e+09 | [1.85, 1.90) | 4.10277e+08 | [3.55, 3.06) | 2.28545e+07 | [5.25, 5.30) | 3.9884e+06 |
| [0.20, 0.25) | 3.61745e+09 | [1.90, 1.95) | 3.34644e+08 | [3.60, 3.65) | 2.21971e+07 | [5.30, 5.35) | 3.50637e+06 |
| [0.25, 0.30) | 3.98637e+09 | [1.95, 2.00) | 2.70411e+08 | [3.65, 3.70) | 2.1078e+07 | [5.35, 5.40) | 3.35139e+06 |
| [0.30, 0.35) | 4.26238e+09 | [2.00, 2.05) | 2.15836e+08 | [3.70, 3.75) | 2.06122e+07 | [5.40, 5.45) | 3.21936e+06 |
| [0.35, 0.40) | 4.46389e+09 | [2.05, 2.10) | 1.76473e+08 | [3.75, 3.80) | 2.00581e+07 | [5.45, 5.50) | 3.40673e+06 |
| [0.40, 0.45) | 4.72023e+09 | [2.10, 2.15) | 1.45358e+08 | [3.80, 3.85) | 1.81843e+07 | [5.50, 5.55) | 2.78167e+06 |
| [0.45, 0.50) | 4.92222e+09 | [2.15, 2.20) | 1.1527e+08 | [3.85, 3.90) | 1.74887e+07 | [5.55, 5.60) | 2.91287e+06 |
| [0.50, 0.55) | 5.03407e+09 | [2.20, 2.25) | 9.90896e+07 | [3.90, 3.95) | 1.66799e+07 | [5.60, 5.65) | 2.92959e+06 |
| [0.55, 0.60) | 5.04208e+09 | [2.25, 2.30) | 8.52773e+07 | [3.95, 4.00) | 1.64523e+07 | [5.65, 5.70) | 2.17844e+06 |
| [0.60, 0.65) | 4.97703e+09 | [2.30, 2.35) | 7.38661e+07 | [4.00, 4.05) | 1.55457e+07 | [5.70, 5.75) | 1.93646e+06 |
| [0.65, 0.70) | 4.92587e+09 | [2.35, 2.40) | 6.44309e+07 | [4.05, 4.10) | 1.5356e+07 | [5.75, 5.80) | 1.90882e+06 |
| [0.70, 0.75) | 4.8751e+09 | [2.40, 2.45) | 5.85384e+07 | [4.10, 4.15) | 1.39368e+07 | [5.80, 5.85) | 1.72019e+06 |
| [0.75, 0.80) | 4.76129e+09 | [2.45, 2.50) | 5.3078e+07 | [4.15, 4.20) | 1.34038e+07 | [5.85, 5.90) | 1.55302e+06 |
| [0.80, 0.85) | 4.58316e+09 | [2.50, 2.55) | 4.90472e+07 | [4.20, 4.25) | 1.24599e+07 | [5.90, 5.95) | 1.41571e+06 |
| [0.85, 0.90) | 4.39217e+09 | [2.55, 2.60) | 4.60699e+07 | [4.25, 4.30) | 1.19725e+07 | [5.95, 6.00) | 1.27656e+06 |
| [0.90, 0.95) | 4.20125e+09 | [2.60, 2.65) | 4.42574e+07 | [4.30, 4.35) | 1.18597e+07 | [6.00, 6.05) | 1.1948e+06 |
| [0.95, 1.00) | 3.97732e+09 | [2.65, 2.70) | 4.28918e+07 | [4.35, 4.40) | 1.13837e+07 | [6.05, 6.10) | 1.01098e+06 |
| [1.00, 1.05) | 3.77124e+09 | [2.70, 2.75) | 4.11151e+07 | [4.40, 4.45) | 1.09077e+07 | [6.10, 6.15) | 969534 |
| [1.05, 1.10) | 3.53281e+09 | [2.75, 2.80) | 3.82788e+07 | [4.45, 4.50) | 1.05582e+07 | [6.15, 6.20) | 810245 |
| [1.10, 1.15) | 3.28751e+09 | [2.80, 2.85) | 3.77446e+07 | [4.50, 4.55) | 9.16137e+06 | [6.20, 6.25) | 659234 |
| [1.15, 1.20) | 3.0546e+09 | [2.85, 2.90) | 3.65919e+07 | [4.55, 4.60) | 9.22129e+06 | [6.25, 6.30) | 546751 |
| [1.20, 1.25) | 2.83217e+09 | [2.90, 2.95) | 3.58925e+07 | [4.60, 4.65) | 8.65399e+06 | [6.30, 6.35) | 511249 |
| [1.25, 1.30) | 2.57803e+09 | [2.95, 3.00) | 3.34044e+07 | [4.65, 4.70) | 7.9764e+06 | [6.35, 6.40) | 391682 |
| [1.30, 1.35) | 2.34652e+09 | [3.00, 3.05) | 3.2049e+07 | [4.70, 4.75) | 7.75966e+06 | [6.40, 6.45) | 302001 |
| [1.35, 1.40) | 2.10236e+09 | [3.05, 3.10) | 3.10074e+07 | [4.75, 4.80) | 7.18408e+06 | [6.45, 6.50) | 276934 |
| [1.40, 1.45) | 1.85976e+09 | [3.10, 3.15) | 3.1785e+07 | [4.80, 4.85) | 6.73098e+06 | [6.50, 6.55) | 205180 |
| [1.45, 1.50) | 1.62091e+09 | [3.15, 3.20) | 2.97035e+07 | [4.85, 4.90) | 6.40431e+06 | [6.55, 6.60) | 162341 |
| [1.50, 1.55) | 1.41211e+09 | [3.20, 3.25) | 2.87819e+07 | [4.90, 4.95) | 6.07857e+06 | [6.60, 6.65) | 124010 |
| [1.55, 1.60) | 1.21925e+09 | [3.25, 3.30) | 2.81035e+07 | [4.95, 5.00) | 5.43618e+06 | [6.65, 6.70) | 82297.6 |
| [1.60, 1.65) | 1.0362e+09 | [3.30, 3.35) | 2.67015e+07 | [5.00, 5.05) | 5.24592e+06 | [6.70, 6.75) | 38330.4 |
| [1.65, 1.70) | 8.73529e+08 | [3.35, 3.40) | 2.65811e+07 | [5.05, 5.1) | 4.93755e+06 | [6.75, 6.80) | 0 |
